# Supplementary material for: Efficient Modelling Across Time of Human Actions and Interactions
Source: arXiv:2110.02120 source file (2021-10-05)
Supplement: Supplementary file 1 [file appendixB.tex]

\usemintedstyle{friendly}

\chapter{Source Code}

\section{Soft Nearest neighbour cyclic consistency}
\label{app:soft_ncc}
\begin{minted}[fontsize=\footnotesize]{python}
import torch

'''
---  S T A R T  O F  F U N C T I O N  S O F T _ N N C  ---
    [About]
        Function takes two tensors both of size (batch x channels x frames
        x height x width) and return a 0-1 tensor for the cyclic consistency
        of the first tensor w.r.t. the second tensor.
        For simplicity we use the following notation in code:
        - b: mini-batch size
        - c: channels
        - f: frames
        - h: height
        - w: width
    [Args]
        - embeddings1: PyTorch Tensor of size 
             (batch x channels x frames x height x width).
        - embeddings2: PyTorch Tensor of size 
             (batch x channels x frames x height x width).
    [Returns]
        - b_consistent: PyTorch Tensor of size (batch)
'''
def soft_nnc(embeddings1,embeddings2):

    # Assume inputs shapes of (b x) x c x f x h x w
    dims_1 = embeddings1.shape
    dims_2 = embeddings2.shape

    # Pooling Height and width to create frame-wise feature representation
    if len(dims_1)>3:
        if (dims_1[-1]>1 or dims_1[-2]>1):
            embeddings1 = F.avg_pool3d(input=embeddings1, 
                                       kernel_size=(1,dims_1[-2],dims_1[-1])
                                       )
        embeddings1=embeddings1.squeeze(-1).squeeze(-1)
    if len(dims_2)>3:
        if (dims_2[-1]>1 or dims_2[-2]>1):
            embeddings2 = F.avg_pool3d(input=embeddings2, 
                                       kernel_size=(1,dims_2[-2],dims_1[-1])
                                       )
        embeddings2=embeddings2.squeeze(-1).squeeze(-1)


    # embeddings1: [b x c x f] --> [f x b x c x 1]
    emb1 = embeddings1.permute(2,0,1).unsqueeze(-1)

    # embeddings2: [b x c x f] --> [f x b x c x f]
    emb2 = embeddings2.unsqueeze(0).repeat(embeddings2.size()[-1],1,1,1)

    # euclidian distance calculation
    distances = torch.abs(emb1-emb2).pow(2)

    # Softmax calculation
    softmax = torch.exp(distances)/torch.exp(torch.sum(distances,dim=-1))
    softmax = softmax.unsqueeze(-1)

    # Soft nearest neighbour calculator (all frames)
    soft_nn = torch.sum(softmax*emb2,dim=-1)

    # Permute [f x b x c] --> [f x b x c x 1]
    soft_nn = soft_nn.unsqueeze(-1)

    # Find points of soft nn in embeddings2
    values,indices = torch.min(torch.abs(soft_nn-emb2).pow(2),dim=-1)

    indices = indices.permute(1,2,0)
    values = values.permute(1,2,0)

    # Get batch-wise T/F values
    nearest_n = embeddings2.scatter_(2,indices,1.)
    b_consistent = embeddings2 - nearest_n

    # [b x c x f] --> [b]
    b_consistent = b_consistent.sum(-1).sum(-1)

    # Non-zero elements are not consistent
    b_consistent[b_consistent==0.] = 1.
    b_consistent[b_consistent!=0.] = 0.

    return b_consistent
\end{minted}

\section{Temporal triplet cosine similarity pooling}
\label{app:cossim}
\begin{minted}[fontsize=\footnotesize]{python}
import torch
import torch.nn.functional as F

'''
---  S T A R T  O F  F U N C T I O N  T E M P O R A L _ C O S S I M _ P O O L  ---
    [About]
        Function that takes as input a `Tensor` x of size 
        (batch x channels x frames x height x width) and
        selects the top k frames with the largest triplet
        dissimilarities with k = floor(frames * r).
        For simplicity we use the following notation in code:
        - b: mini-batch size
        - c: channels
        - f: frames
        - h: height
        - w: width
    [Args]
        - x: PyTorch Tensor of size 
             (batch x channels x frames x height x width).
    [Returns]
        - x: PyTorch Tensor of size 
            (batch x channels x floor(frames*r) x height x width)
'''
def temporal_cossim_pool(x, r=0.5):

    #Get shape
    dims = x.shape

    # Calculate spatially global pooled tensor 
    #[b x c x f x h x w] -> [b x c x f x 1 x 1]
    gp_x = F.avg_pool3d(x,kernel_size=(1,dims[-2],dims[-1])).squeeze(-1).squeeze(-1)

    # frame pair-wise cosine similarity: ceil(cos(f_{i},f_{i+1}),1e-4)**2
    distances = F.cosine_similarity(x1=gp_x[...,:-1],
                                    x2=gp_x[...,1:],
                                    eps=1e-4).pow(2).unsqueeze(1)
    triplet_distance_mean = F.avg_pool1d(distances,kernel_size=2,stride=1)

    # Topk cosine sim triplet indices
    tk = math.floor(dims[-3]*r)
    _,max_k = torch.topk(triplet_distance_mean.squeeze(1),
                         k=math.floor(dims[-3]/2),
                         largest=True,
                         dim=-1)
    # Correspondence with tensor X's indices
    max_k += 1
    max_k,_ = torch.sort(max_k,descending=False)

    # Change shape [b x c x f x h x w] -> [b x f x c x h x w]
    x = x.permute(0,2,1,3,4)
    # Batch-wise frame indices selection
    x = x[torch.arange(x.shape[0])[:,None],max_k]
    # Revert shape and return
    # [b x floor(f/2) x c x h x w] -> [b x c x floor(f/2) x h x w]
    return x.permute(0,2,1,3,4)
\end{minted}

\section{Frame augmentation}
\label{app:frame_aug}
\begin{minted}[fontsize=\footnotesize]{python}
import numpy as np
import imgaug.augmenters as iaa

sometimes_aug = lambda aug: iaa.Sometimes(0.4, aug)
sometimes_seq = lambda aug: iaa.Sometimes(0.8, aug)

frame_transform = iaa.Sequential([
    iaa.Resize({"shorter-side": 320, 
                "longer-side":"keep-aspect-ratio"}),
    iaa.CropToFixedSize(width=256, height=256, 
                        position='uniform'),
    sometimes_seq(iaa.Sequential([
        sometimes_aug(iaa.GaussianBlur(sigma=[0.1,0.2,0.3])),
        sometimes_aug(iaa.Add((-5, 15), per_channel=True)),
        sometimes_aug(iaa.AverageBlur(k=(1,2))),
        sometimes_aug(iaa.Multiply((0.8, 1.2))),
        sometimes_aug(iaa.GammaContrast((0.85,1.15),
                                        per_channel=True)),
        sometimes_aug(iaa.AddToHueAndSaturation((-16, 16), 
                                                per_channel=True)),
        sometimes_aug(iaa.LinearContrast((0.85, 1.115))),
        sometimes_aug(iaa.OneOf([
            iaa.PerspectiveTransform(scale=(0.02, 0.05), 
                                     keep_size=True),
            iaa.Rotate(rotate=(-10,10)),
        ]))
    ])),
    iaa.Fliplr(0.5)
])
\end{minted}
