# Supplementary material for: Efficient Modelling Across Time of Human Actions and Interactions
Source: arXiv:2110.02120 source file (2021-10-05)
Supplement: Supplementary file 2 [file appendixA.tex]

\chapter{The First Appendix}
\label{app:first-app}
\kant[20-21] % Dummy text
\section{First Section}
\kant[22]    % Dummy text
\section{Second Section}
\kant[23-24] % Dummy text
